# Supplementary material for: Is it worth it? Comparing six deep and classical methods for unsupervised anomaly detection in time series
Source: arXiv:2212.11080 source file (2023-02-02)
Supplement: Supplementary file 1 [file appendix.tex]

\appendixtitles{no} % Leave argument "no" if all appendix headings stay EMPTY (then no dot is printed after "Appendix A"). If the appendix sections contain a heading then change the argument to "yes".
\appendixstart
\appendix
\section[\appendixname~\thesection]{}

\subsection[\appendixname~\thesubsection]{}
\label{appendix:anomaly_types}
\input{sections/appendix/anomaly_types_examples}

\subsection[\appendixname~\thesubsection]{}
\label{appendix:parameters}
\input{sections/appendix/hyperparams}

\subsection[\appendixname~\thesubsection]{}
\label{appendix:stds_by_anomaly_type}
\input{sections/appendix/anomaly_types_stddevs}
